# Supplementary material for: Constant-Time Predictive Distributions for Gaussian Processes
Source: arXiv:1803.06058 source file (2018-06-20)
Supplement: Supplementary file 1 [file lanczos.tex]

\section{The Lanczos Algorithm}
\label{sec:lanczos}

\gp{More details here, as necessary}

\paragraph{Re-orthogonalization.}
\gp{TODO.}
